# Supplementary material for: Quantified Facial Expressiveness for Affective Behavior Analytics
Source: arXiv:2110.01758 source file (2021-10-07)
Supplement: Supplementary file 1 [file appendix.tex]

\clearpage
\section*{Appendix}

\begin{table}[h]
 \caption{A brief introduction to the facial action units \cite{ekman1976measuring} evaluated in this work. %\footnote{Please see this iMotions webpage for GIF \url{https://rb.gy/qbt8lb}}.
 }
  \centering
  \begin{tabular}{L{0.5cm}L{2.5cm}L{0.5cm}L{3cm}}
    \toprule
     \multicolumn{2}{c}{\textbf{Upper}} & \multicolumn{2}{c}{\textbf{Lower}} \\
    \cmidrule(r){1-2} \cmidrule(r){3-4}
    
    AU & Description & AU & Description \\
    \midrule
    % 1 & 2 & 4 & 5 & 6 & 7 & 9 & 10 & 12 & 14 & 15 & 17 & 20 & 23 & 25 & 26 & 28 & 45 \\ 
    1 & Inner brow raiser & 10 & Upper lip raiser  \\
    2 & Outer brow raiser &  12 & Lip corner puller \\
    4 & Brow lowerer & 14 & Dimpler \\ 
    5 & Upper lid raiser & 15 & Lip corner depressor \\ 
    6 & Cheek raiser & 17 & Chin raiser \\
    7 & Lid tightener & 20 & Lip stretcher \\
    9 & Nose wrinkler & 23 & Lip tightener \\
    45 & Blink & 25 & Lips part \\ 
     & & 26 & Jaw drop \\
     & & 28 & Lip suck \\ 

    \bottomrule
  \end{tabular}
  \label{tab:FACS_desp}
\end{table}

\begin{table}[h]
 \caption{Facial AUs and associated discrete emotion/affect/expression category \cite{barrett2019emotional}.  Category = Emotion / Affect / Expression. %\footnote{Please see this iMotions webpage for GIF \url{https://rb.gy/qbt8lb}}.
 }
  \centering
  \begin{tabular}{L{2cm}L{3cm}L{3cm}}
    \toprule
    Category & Associated AUs & Studied AUs\\
    \midrule
    Amusement & [6, 7, 12, 25, 26, \textcolor{gray}{53}] & [6, 7, 12, 25, 26]\\ 
    Anger & [4, 5, 17, 23, \textcolor{gray}{24}] & [4, 5, 17, 23] \\ 
    Confusion & [4, 7, \textcolor{gray}{56}] & [4, 7] \\ 
    Disgust & [7, 9, \textcolor{gray}{19}, 25, 26] & [7, 9, 25, 26] \\ 
    Embarrassment & [7, 12, 15, \textcolor{gray}{52, 54, 64}] & [7, 12, 15] \\ 
    Fear & [1, 2, 4, 5, 7, 20, 25] & [1, 2, 4, 5, 7, 20, 25] \\ 
    Happiness & [6, 7, 12, 25, 26] & [6, 7, 12, 25, 26] \\ 
    Interest & [1, 2, 12] & [1, 2, 12]  \\
    Pain & [4, 6, 7, 9, 17, \textcolor{gray}{18}, 23, \textcolor{gray}{24}] or [4, 6, 9, 10, 25, 43] \cite{werner2019automatic}  & [4, 6, 7, 9, 17, 23]\\ 
    Sadness & [1, 4, 6, 15, 17] & [1, 4, 6, 15, 17] \\ 
    Surprise & [1, 2, 5, 25, 26] & [1, 2, 5, 25, 26] \\ 
    Sympathy & [1, 17, \textcolor{gray}{24, 57}] & [1, 17] \\
    \bottomrule
  \end{tabular}
  \label{tab:FACS_cat_assoc}
\end{table}
