# Supplementary material for: Quantified Facial Expressiveness for Affective Behavior Analytics
Source: arXiv:2110.01758 source file (2021-10-07)
Supplement: Supplementary file 2 [file supplement.tex]

\appendix
\section{Additional experiments}

\begin{table*}
 \caption{Percentage (\%) of video segments for which temperature Granger-caused pain in terms of pain level and pain expressiveness. We set the significance level $\alpha = 0.05$. $\tau_{pain}$ QFE score computed for pain expression; \textbf{PVSP} = percentage of video segment passed; \textbf{ALL} denotes passed all four tests. 
 }
  \centering
  \begin{tabular}{L{1cm}L{1cm}|C{1cm}C{1cm}C{1cm}C{1cm}C{1cm}|C{1cm}C{1cm}C{1cm}C{1cm}C{1cm}}
    \toprule
    
    \multicolumn{2}{c}{Lag} &  \multicolumn{5}{c}{\textbf{GC (Temperature) $\longrightarrow$ PL}} & \multicolumn{5}{c}{\textbf{GC (Temperature) $\longrightarrow$ $\tau_{pain}$ }} \\
     \cmidrule(r){1-2} \cmidrule(r){3-7} \cmidrule(r){8-12} 
     Time (sec.) & \# of frames &	PVSP LR test $\chi^{2}$	& PVSP params F test & PVSP SSR $\chi^{2}$ &	PVSP SSR F test F	& ALL & PVSP LR test $\chi^{2}$	& PVSP params F test & PVSP SSR $\chi^{2}$ &	PVSP SSR F test F	& ALL\\
    \midrule
    % \hline
    1 & 5 & 50.8 & 47.8 & 52.8 & 47.8 & 47.8 & 11.0 & 10.0 & 11.0 & 10.0 & 10.0 \\ 
    2 & 10 & 87.7 & 82.8 & 89.3 & 82.8 & 82.8 & 16.0 & 14.0 & 17.0 & 14.0 & 14.0 \\ 
    3 & 15 & 90.4 & 85.2 & 92.1 & 85.2 & 85.2 & 20.0 & 15.0 & 22.0 & 15.0 & 15.0 \\ 
    4 & 20 & 99.5 & 99.0 & 99.7 & 99.0 & 99.0 & 26.0 & 17.0 & 30.0 & 17.0 & 17.0 \\ 
    5 & 25 & 100.0 & 100.0 & 100.0 & 100.0 & 100.0 & 33.0 & 21.0 & 39.0 & 21.0 & 21.0 \\ 
    6 & 30 & 100.0 & 100.0 & 100.0 & 100.0 & 100.0 & 39.0 & 23.0 & 47.0 & 23.0 & 23.0 \\ 
    7 & 35 & 100.0 & 100.0 & 100.0 & 100.0 & 100.0 & 46.0 & 23.0 & 57.0 & 23.0 & 23.0 \\ 
    8 & 40 & 100.0 & 100.0 & 100.0 & 100.0 & 100.0 & 54.0 & 21.0 & 65.0 & 21.0 & 21.0 \\ 
    9 & 45 & 100.0 & 99.8 & 100.0 & 99.8 & 99.8 & 59.0 & 18.0 & 73.0 & 18.0 & 18.0 \\ 
    10 & 50 & 100.0 & 99.4 & 100.0 & 99.4 & 99.4 & 67.0 & 15.0 & 80.0 & 15.0 & 15.0 \\ 
    11 & 55 & 100.0 & 98.4 & 100.0 & 98.4 & 98.4 & 75.0 & 13.0 & 88.0 & 13.0 & 13.0 \\ 
    12 & 60 & 100.0 & 95.8 & 100.0 & 95.8 & 95.8 & 84.0 & 10.0 & 94.0 & 10.0 & 10.0 \\ 
    13 & 65 & 100.0 & 94.7 & 100.0 & 94.7 & 94.7 & 91.0 & 7.0 & 97.0 & 7.0 & 7.0 \\ 
    14 & 70 & 100.0 & 93.7 & 100.0 & 93.7 & 93.7 & 95.0 & 5.0 & 98.0 & 5.0 & 5.0 \\ 
    15 & 75 & 100.0 & 89.4 & 100.0 & 89.4 & 89.4 & 98.0 & 4.0 & 99.0 & 4.0 & 4.0 \\ 
    16 & 80 & 99.9 & 83.4 & 100.0 & 83.4 & 83.4 & 99.0 & 3.0 & 100.0 & 3.0 & 3.0 \\ 
    17 & 85 & 99.9 & 76.4 & 99.9 & 76.4 & 76.4 & 99.0 & 3.0 & 100.0 & 3.0 & 3.0 \\ 
    18 & 90 & 99.7 & 67.6 & 99.7 & 67.6 & 67.6 & 100.0 & 3.0 & 100.0 & 3.0 & 3.0 \\ 
    19 & 95 & 99.6 & 54.6 & 99.6 & 54.6 & 54.6 & 100.0 & 3.0 & 100.0 & 3.0 & 3.0 \\
    \bottomrule
  \end{tabular}
  \label{tab:GC_res_v2}
\end{table*}
